# Supplementary material for: Ultrafast Transient Dynamics of Adsorbates on Surfaces Deciphered: The Case of CO on Cu(100)
Source: arXiv:1806.10492 ancillary file (2019-01-11)
Supplement: Supplementary file 1 [file SM.pdf]

# Supplemental Material: Ultrafast Transient Dynamics of Adsorbates on Surfaces Deciphered: The Case of CO on Cu(100)

D. Novko,[1,2,*] J. C. Tremblay,[3] M. Alducin,[4,2] and J. I. Juaristi[5,4,2]

[1] *Center of Excellence for Advanced Materials and Sensing Devices, Institute of Physics, Bijenička 46, 10000 Zagreb, Croatia*

[2] *Donostia International Physics Center (DIPC), Paseo Manuel de Lardizabal 4, 20018 Donostia-San Sebastián, Spain*

[3] *Institut für Chemie und Biochemie, Freie Universität Berlin, Takustr. 3, 14195 Berlin, Germany*

[4] *Centro de Física de Materiales CFM/MPC (CSIC-UPV/EHU), Paseo Manuel de Lardizabal 5, 20018 Donostia-San Sebastián, Spain*

[5] *Departamento de Física de Materiales, Facultad de Químicas UPV/EHU, Apartado 1072, 20080 Donostia-San Sebastián, Spain*

[*] dino.novko@gmail.com

## S1. TWO TEMPERATURE MODEL

Excitation of the electronic system in metals by ultrafast laser pulses and its subsequent relaxation into the lattice degrees of freedom (electron-phonon coupling) can be simulated by means of the two temperature model (TTM) [S1]. In this model, the excited electrons and phonons are described in terms of nonthermal electron $T_e$ and lattice $T_l$ temperatures that satisfy the following coupled equations [S2–S7]

$$C_e(T_e)\frac{\partial T_e}{\partial t} = \nabla_z \cdot (\kappa \nabla_z \cdot T_e) - G(T_e)(T_e - T_l) + S(z,t) \tag{S1}$$

and

$$C_l(T_l)\frac{\partial T_l}{\partial t} = G(T_e)(T_e - T_l), \tag{S2}$$

where $C_e$ and $C_l$ are the electron and lattice heat capacities, respectively, $\kappa$ is the thermal conductivity of electrons, and $G$ is the TTM electron-phonon coupling constant (not to be confused with the standard electron-phonon coupling constant $\lambda$). The coupling of the metal electrons with the pump laser, which is acting as the heat source, is described by the last term in Eq. S1, i.e., $S(z,t) = I(t)e^{-z/\delta}/\delta$, where $I(t)$ is the intensity of the absorbed fraction of the laser pulse (with a Gaussian profile) and $\delta$ is the penetration depth. Since we are dealing with high but not extreme temperatures, we adopt the usual approximations for the TTM input functions [S2, S3, S7]: $C_e(T_e) = \beta T_e$, $C_l(T_l) =$ const., and $\kappa = \kappa_0 T_e/T_l$. Nevertheless, with the exception of $\kappa_0$ and $S$, we calculate all the input parameters using density functional and density functional perturbation theories [S8] (see Sec. S3 for computational details). Specifically, $C_e$ and $C_l$ are first calculated as [S6]

$$C_e(T_e) = \int_{-\infty}^{\infty} d\varepsilon N_e(\varepsilon)\varepsilon \frac{\partial f(\varepsilon;T_e)}{\partial T_e}, \tag{S3}$$

$$C_l(T_l) = \int_0^{\infty} d\omega N_b(\omega)\omega \frac{\partial n_b(\omega;T_l)}{\partial T_l}, \tag{S4}$$

where $N_e$ and $N_b$ are the electron and phonon density of states, while $f$ and $n_b$ are the Fermi-Dirac and Bose-Einstein distribution functions, respectively. The $C_e$ values calculated with Eq. S3 for different $T_e$ are then fitted to a linear function $\beta T_e$ in order to extract $\beta$, while for $C_l$ we take the corresponding value of Eq. S4 at $k_B T_l \gg \max\{\omega_\nu\}$. Since robust

*ab initio* calculations of $G(T_e)$ for copper show that this function varies slowly with $T_e$ up to about 6000 K [S6], we opt for calculating a temperature-independent $G$ as [S2]

$$G = \pi k_B \lambda \left\langle \omega^2 \right\rangle N_e(\varepsilon_F)/\hbar, \tag{S5}$$

where $\varepsilon_F$ is the Fermi energy and $\lambda \langle \omega^2 \rangle$ is the second moment of the phonon spectrum multiplied by the electron-phonon coupling constant. Even though we treat $G$ in Eqs. S1 and S2 as a constant with respect to temperature changes, we acknowledge that it could vary with $T_e$ and even $T_l$ because the CO/Cu(100) system has high-energy internal stretch CO modes that are activated only at high temperatures ($\omega_{\mathrm{IS}}/k_B \approx 3000\,\mathrm{K}$). In all our simulations, we use the following formula for $\lambda \langle \omega^2 \rangle$ in order to get the final value of $G$ [S2]

$$\lambda \left\langle \omega^2 \right\rangle = 2 \int d\Omega \Omega^2 \alpha^2 F(\Omega) \frac{n_b(T_e) - n_b(T_l)}{k_B T_e - k_B T_l}. \tag{S6}$$

The phonon spectral function weighted with electron-phonon coupling strengths, i.e., the Eliashberg function, is denoted as $\alpha^2 F$. Before introducing representative temperatures into Eq. S6 for obtaining a final value of $G$, we first calculate $\lambda \langle \omega^2 \rangle$ for $T_e, T_l \gg \Omega/k_B$. In that case we get $\lambda \langle \omega^2 \rangle = 43\,\mathrm{meV}^2$ ($G = 0.74 \times 10^{17}\,\mathrm{W/m^3K}$) and $\lambda \langle \omega^2 \rangle = 208\,\mathrm{meV}^2$ ($G = 3.6 \times 10^{17}\,\mathrm{W/m^3K}$) for Cu(100) and CO/Cu(100), respectively. Figure S1 shows $\lambda \langle \omega^2 \rangle$ for a representative range of laser-induced $T_e$ and $T_l$ temperatures, where the integral in Eq. S6 is performed up to some finite $\omega$ value. The final result of $\lambda \langle \omega^2 \rangle$ is obtained for $\omega > \omega_{\mathrm{IS}}$, i.e., above $\approx 2080\,\mathrm{cm}^{-1}$. We see that $\lambda \langle \omega^2 \rangle$ for CO/Cu(100) varies strongly with temperature. For Cu(100) the changes are minor (not shown). The final $G$ used in the main text is calculated with Eq. S6 for $T_e = 5000\,\mathrm{K}$ and $T_l = 400\,\mathrm{K}$. An improvement upon

TABLE S1. The TTM input parameters calculated with density functional and density functional perturbation theories [S8] [with exception of $\kappa_0$, which is taken from Ref. [S3]].

| | CO/Cu(100) | Cu(100) |
|---|---|---|
| $\lambda$ | 0.18 | 0.13 |
| $\lambda \langle \omega^2 \rangle$ [meV$^2$] | 187 | 43 |
| $G \times 10^{17}$ [W/m$^3$K] | 3.2 | 0.7 |
| $\beta$ [J/m$^3$K$^2$] | 97 | 97 |
| $C_l \times 10^6$ [J/m$^3$K] | 3.4 | 2.8 |
| $\kappa_0$ [W/mK] | 428 | 428 |

this model would be to integrate numerically Eqs. S1 and S2 with a $G$ factor depending on $T_e$ and $T_l$ explicitly [S6, S9]. In addition, introducing the phonon-mode-dependent $G$ factor would constitute an upgrade of the model [S10]. However, we expect that the accompanying corrections to the final results would be within the error bars of the experimental data. Table S1 summarizes all the TTM input parameters for CO/Cu(100) and Cu(100) that have been used in Eqs. S1 and S2 to obtain $T_e$ and $T_l$ as a function of time.

### S1.1. Impact of the CO modes on total heat transfer

Figure S2 displays the TTM results for $T_e(t)$ and $T_l(t)$ when a 400 nm laser pump, with 170 J/m$^2$ absorbed fluence and 150 fs duration, excites the surface electrons. In order to simulate the laser-induced dynamics of adsorbates on surfaces, the TTM is frequently adopted along with the Langevin equation for the adsorbates [S11, S12], whereby only the surface motions are contributing to $T_l(t)$. In our theoretical framework, $T_l(t)$ should additionally contain the contribution from the CO modes (summation over $\nu'$ modes in Eq. S12 goes

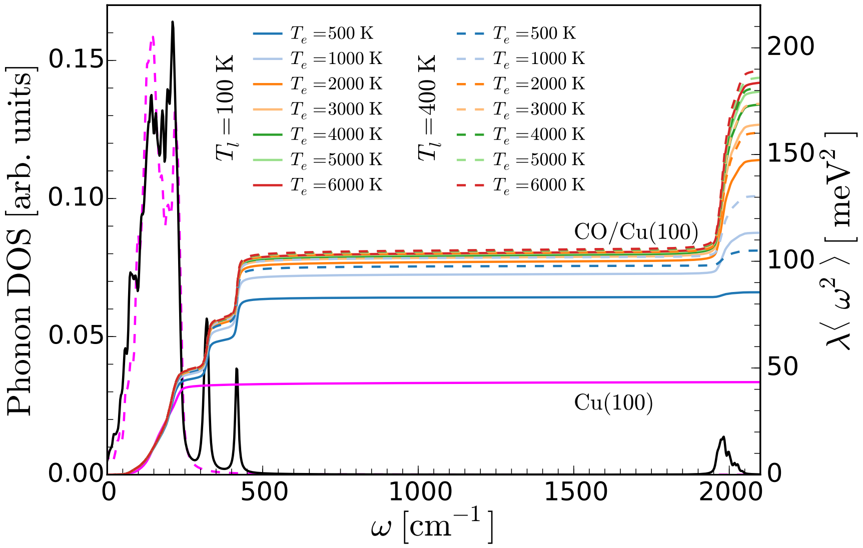


FIG. S1. Left y-axis: phonon density of states for CO/Cu(100) (black) and Cu(100) (magenta). Right y-axis: second moment of the phonon spectrum multiplied by the electron-phonon coupling constant $\lambda\langle\omega^2\rangle$ for CO/Cu(100) (various colors for various $T_e$ and $T_l$) and Cu(100) (magenta), where integral in Eq. S6 is performed up to a finite $\omega$ value. The final results of $\lambda\langle\omega^2\rangle$ are obtained for $\omega > \omega_{\rm IS}$.

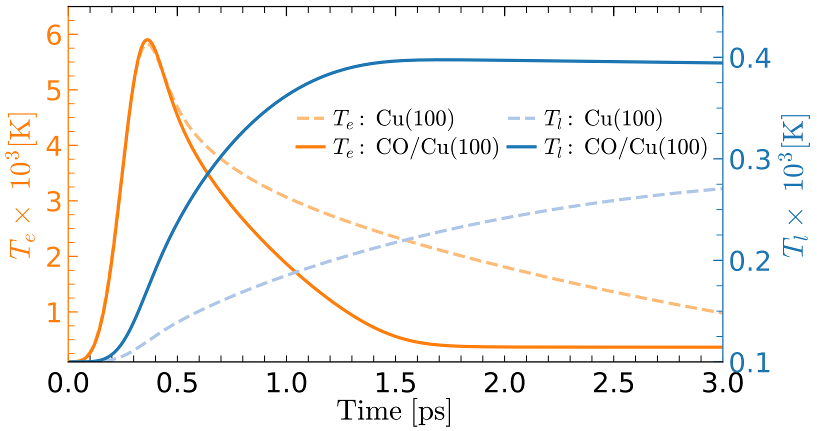


FIG. S2. Electron $T_e(t)$ and lattice $T_l(t)$ temperatures as a function of time for a 400 nm laser pump, with 170 J/m$^2$ absorbed fluence and 150 fs duration. Full and dashed lines represent the results when either all or only surface modes of CO/Cu(100) are included in TTM, respectively.

over all modes in the system). This is somehow similar to those cases where the effective adsorbate temperature is considered via a complementary heat transfer equation for the adsorbates (sometimes called the three temperature model) [S13–S15]. Figure S2 shows that the energy transfer between the laser-induced hot electrons and phonons changes notably when along with the surface modes the TTM also includes the CO modes (compare full and dashed lines). First, after the electrons are heated up to the maximum temperature of about 5800 K, they dissipate their energy more rapidly to phonons when the CO modes are active. The reason is that the TTM electron-phonon coupling constant $G$ is larger for CO/Cu(100) than it is for Cu(100) (see Table S1). Also, since more modes are included, $T_l(t)$ is higher for CO/Cu(100) than for Cu(100). In principle, all these differences in $T_e$ and $T_l$ remark the importance of including all active modes to correctly describe the electron and phonon distributions in our formalism. Nevertheless, the differences obtained in the calculated transient frequency and linewidth changes when using the Cu(100) electronic and lattice temperatures are smaller than the experimental error bars (not shown).

## S2. PHONON FREQUENCY SHIFT AND LINEWIDTH

The nonadiabatic phonon spectral function that includes the electron-phonon interaction can be evaluated by means of many-body perturbation theory and has the following

form [S16–S18]

$$A_\nu(\mathbf{q},\omega) = \frac{1}{\pi}\mathrm{Im}\left[\frac{2\omega_{\mathbf{q}\nu}}{\omega^2 - \omega_{\mathbf{q}\nu}^2 - 2\omega_{\mathbf{q}\nu}\pi_\nu(\mathbf{q},\omega)}\right], \tag{S7}$$

where $\nu$ and $\mathbf{q}$ are the phonon band index and momentum, respectively, and $\omega_{\mathbf{q}\nu}$ is the adiabatic phonon frequency. The latter is usually calculated within density functional perturbation theory (DFPT) [S8] and, in such a case, it already includes corrections ascribed to the static electron-phonon interaction. All the information about nonadiabatic corrections due to the electron-phonon coupling is contained in the phonon self-energy $\pi_\nu(\mathbf{q},\omega)$ [S19, S20]. Specifically, its real part renormalizes the phonon frequency because of the nonadiabatic coupling,

$$\omega^2 - \omega_{\mathbf{q}\nu}^2 = 2\omega_{\mathbf{q}\nu}\mathrm{Re}\left[\pi_\nu(\mathbf{q},\omega) - \pi_\nu(\mathbf{q},0)\right], \tag{S8}$$

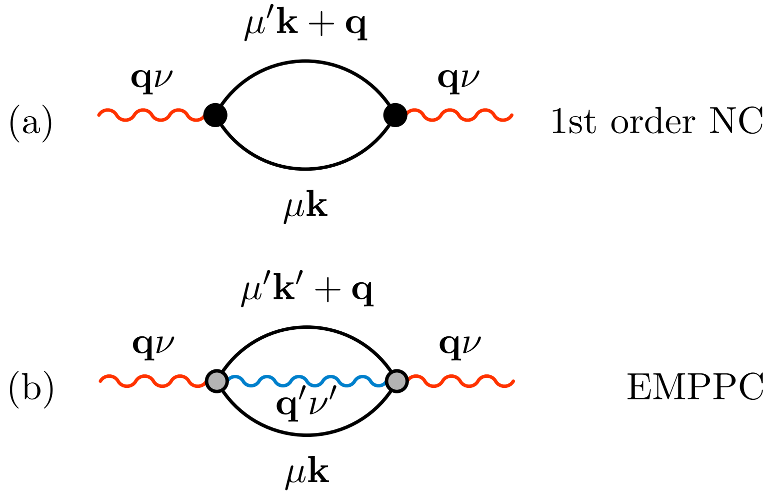


FIG. S3. (a) First-order nonadiabatic coupling term for the phonon propagator, where the $(\mathbf{q},\nu)$ phonon mode is coupled to the noninteracting $(\mu,\mathbf{k})$ and $(\mu,\mathbf{k}+\mathbf{q})$ electron-hole pairs. (b) Electron-mediated phonon-phonon (i.e., second-order nonadiabatic) coupling term for the phonon propagator, where the $(\mathbf{q},\nu)$ phonon mode is coupled to the all other $(\mathbf{q}',\nu')$ phonon modes available in the system via the $(\mu,\mathbf{k})$ and $(\mu,\mathbf{k}+\mathbf{q})$ electron-hole pairs. Black circle represents the electron-phonon coupling function $|g_\nu(\mathbf{k})|^2$, while gray circle is the effective coupling function $|g_\nu(\mathbf{k})|^2|g_{\nu'}(\mathbf{k}')|^2$. In our case $\mathbf{q}\approx\mathbf{0}$, $\nu=\mathrm{IS}$, and $\nu'=\mathrm{Cu,FT,FR,ES,IS}(\mathbf{q}'>\mathbf{0})$ (see also Ref. [S16]).

while its imaginary part gives the corresponding phonon linewidth,

$$\gamma_{\mathbf{q}\nu} = -2\mathrm{Im}\,\pi_\nu(\mathbf{q},\omega). \tag{S9}$$

In Eq. S8 the last term $\pi_\nu(\mathbf{q},0)$ must be included in case of using the DFPT $\omega_{\mathbf{q}\nu}$ that accounts already for the static electron-phonon interaction [S17]. Nonadiabatic corrections to the phonon self-energy are usually small compared to the adiabatic energy (i.e., $\omega-\omega_{\mathbf{q}\nu} \ll \omega_{\mathbf{q}\nu}$), which means that Eq.S8 can be approximated as $\omega-\omega_{\mathbf{q}\nu} \approx \mathrm{Re}\left[\pi_\nu(\mathbf{q},\omega)-\pi_\nu(\mathbf{q},0)\right]$ [S17].

In order to simulate the vibrational spectra probed by infrared light, we focus on the long wavelength part of the phonon self-energy, i.e., $\pi_\nu(\mathbf{q}\approx 0,\omega)\equiv\pi_\nu(\omega)$. In this case, the two dominating terms are the first-order interband and the second-order intraband phonon self-energies [S16, S17] (see Fig. S3), i.e.,

$$\pi_\nu(\omega) \approx \pi_\nu^{[1],\mathrm{inter}}(\omega)+\pi_\nu^{[2],\mathrm{intra}}(\omega). \tag{S10}$$

The interband contribution describes the direct (i.e., momentum-conserving, $\mathbf{k}=\mathbf{k}'$) electron excitations between two different electronic bands and reads [see Fig S3(a)] [S16, S17]

$$\pi_\nu^{[1],\mathrm{inter}}(\omega;T_e) = \sum_{\mu\neq\mu'\mathbf{k}} \left|g_\nu^{\mu\mu'}(\mathbf{k},0)\right|^2 \frac{f(\varepsilon_{\mu\mathbf{k}};T_e)-f(\varepsilon_{\mu'\mathbf{k}};T_e)}{\omega+i\eta+\varepsilon_{\mu\mathbf{k}}-\varepsilon_{\mu'\mathbf{k}}}. \tag{S11}$$

Here an electron and a hole with energies $\varepsilon_{\mu\mathbf{k}}$ and $\varepsilon_{\mu'\mathbf{k}}$, respectively, interact with a single phonon mode $\nu$ via the electron-phonon coupling function $g_\nu^{\mu\mu'}(\mathbf{k},0)$. Since this is a first-order electronic excitation process, the temperature dependence only enters through the Fermi-Dirac distribution function $f(\varepsilon_{\mu\mathbf{k}};T_e)=1/(1+e^{(\varepsilon_{\mu\mathbf{k}}-\varepsilon_F)/k_BT_e})$. An increase in $T_e$ results in the skewing of the electron and hole distributions (i.e., nonthermal charge transfer to unoccupied states, see Fig. 1 in the main text), which in turn changes the intensity of the phonon renormalization Eq. S8 and linewidth Eq. S9. The intraband contribution contains information on indirect (i.e., momentum-non-conserving, $\mathbf{k}\neq\mathbf{k}'$) electron excitations where electrons and holes, excited by the studied phonon mode $(\mathbf{q}\approx 0,\nu)$, undergo further scattering with other available phonons $(\mathbf{q}',\nu')$ [see Fig S3(b)] [S16]. In other words, this term describes electron-mediated phonon-phonon coupling (EMPPC) mechanisms and can be written as

$$\pi_\nu^{[2],\mathrm{intra}}(\omega;T_e,T_l) = -\sum_{\mu\mu'\mathbf{k}\nu'\mathbf{k}'} \left|g_\nu^{\mu\mu}(\mathbf{k},0)\right|^2 \left[1-\frac{g_\nu^{\mu'\mu'}(\mathbf{k}',0)}{g_\nu^{\mu\mu}(\mathbf{k},0)}\right] \left|g_{\nu'}^{\mu\mu'}(\mathbf{k},\mathbf{q}')\right|^2$$
$$\times\sum_{s,s'=\pm1}\frac{s\left[n_b(s\omega_{\mathbf{q}'\nu'};T_l)+f(s'\varepsilon_{\mu'\mathbf{k}'};T_e)\right]\left[f(\varepsilon_{\mu\mathbf{k}};T_e)-f(\varepsilon_{\mu'\mathbf{k}'}-s's\omega_{\mathbf{q}'\nu'};T_e)\right]}{\omega\left[\omega+i\eta+s'(\varepsilon_{\mu\mathbf{k}}-\varepsilon_{\mu'\mathbf{k}'})+s\omega_{\mathbf{q}'\nu'}\right]\left[\varepsilon_{\mu\mathbf{k}}-(\varepsilon_{\mu'\mathbf{k}'}-s's\omega_{\mathbf{q}'\nu'})\right]}. \tag{S12}$$

Due to the two successive electron-phonon couplings – the first one including the single mode under consideration and the second one all available modes in the system – the second-order intraband term $\pi_\nu^{[2],\mathrm{intra}}$ depends on both $T_e$ and $T_l$ via $f(\varepsilon_{\mu\mathbf{k}};T_e)$ and the Bose-Einstein distribution function $n_b(s\omega_{\mathbf{q}'\nu'};T_l)$, respectively.

Finally, by combining Eqs. S11 and S12 with the TTM, i.e., Eqs. S1 and S2, we get an implicit time-dependence of the nonadiabatic phonon frequency and linewidth, via the time-dependent electron and phonon temperatures. The final results presented in the main text are the relative changes with respect to $t = 0$, when $T_e = T_l = 100\,\mathrm{K}$, i.e.,

$$\delta\omega_\nu \equiv \mathrm{Re}\,\pi_\nu(\omega;t) - \mathrm{Re}\,\pi_\nu(\omega;0) \tag{S13}$$

and

$$\delta\gamma_\nu \equiv -2\mathrm{Im}\,\pi_\nu(\omega;t) + 2\mathrm{Im}\,\pi_\nu(\omega;0). \tag{S14}$$

As a final remark, note that the adiabatic phonon frequency is also expected to change with $T_e$. Therefore, in using Eq. S13 we are carefully taking into account that the frequency change measured in experiments also includes this effect.

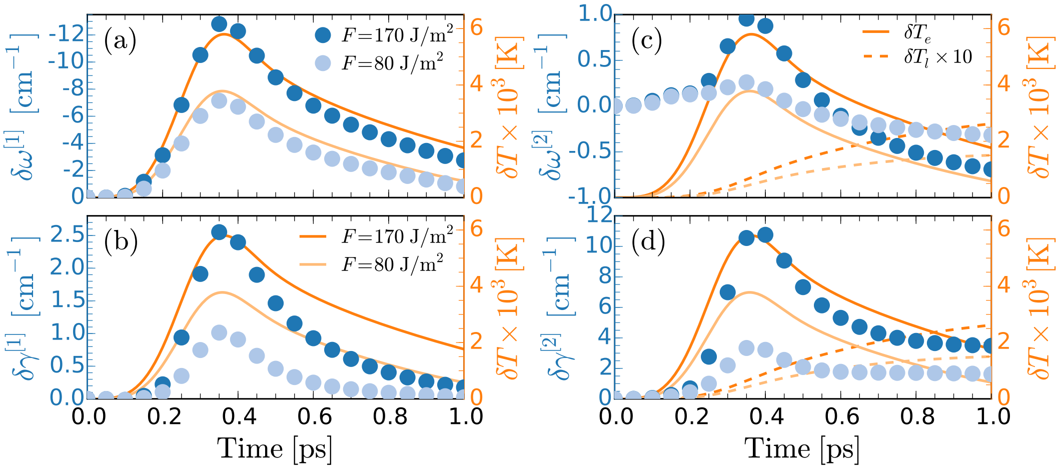


FIG. S4. Time-dependent spectral changes of the CO internal stretch mode on Cu(100) attributed to (a) $\delta\omega^{[1]}$, (b) $\delta\gamma^{[1]}$, (c) $\delta\omega^{[2]}$, and (d) $\delta\gamma^{[2]}$ for two different absorbed fluences $F$ (blue and light blue circles). The right y-axis shows the corresponding temperature changes (orange and light orange).

### S2.1. Correlation between temperatures and spectral changes

The existing correlation between the first- and second-order changes of the CO IS mode and the electron $\delta T_e$ and lattice $\delta T_l$ temperature changes is clearly observed in Fig. S4. Regarding the NC contribution, $\delta\omega^{[1]}$ and $\delta\gamma^{[1]}$ nicely follow the time dependence of $\delta T_e$. In particular, each $\delta\omega^{[1]}$ curve runs almost on top of its corresponding $\delta T_e$ and remarks that there exists an almost linear dependence of the form $\delta\omega^{[1]} \propto -\delta T_e$. The observed redshift can be interpreted as a softening of the C–O interaction caused by the charge transfer to the antibonding $\pi^*$-like orbital as $T_e$ increases, as also suggested by other authors [S21].

As for the EMPPC contribution, the corresponding spectral changes, i.e., $\delta\omega^{[2]}$ and $\delta\gamma^{[2]}$, are affected by the time evolution of both $\delta T_e$ and $\delta T_l$. In fact, $\delta\gamma^{[2]}$ increases up to a maximum value at around $t = 0.4$ ps due to the increase of $T_e$ but, instead of following the subsequent $T_e$ decrease, it goes to a finite value for $t > 0.6$ ps since $\delta T_l$ becomes considerable at longer times. The explicit temperature dependence of $\delta\gamma^{[2]}$ can be observed in Fig. S5. In $\delta\omega^{[2]}$ the effects of $T_e$ and $T_l$ are opposite and compete, i.e., the increase of $T_e$ induces a positive (blue) shift $\delta\omega^{[2]}$, while the increase of $T_l$ induces a negative (red) shift $\delta\omega^{[2]}$ (see Fig. S5). Such a non-monotonous behavior is reflected in a positive $\delta\omega^{[2]}$ at around 0.4 ps, when $T_e \gg T_l \approx 100$ K, and a negative $\delta\omega^{[2]}$ after around 0.6 ps, when $T_e > T_l > 100$ K.

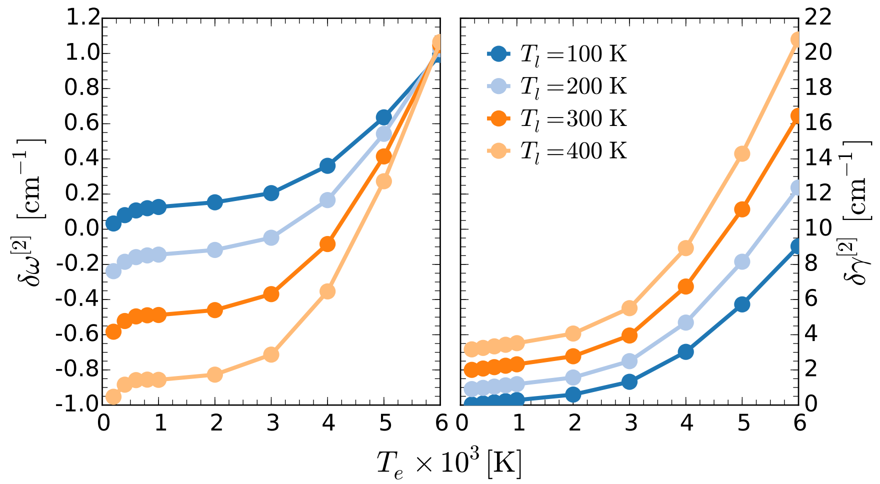


FIG. S5. The EMPPC contribution to frequency $\delta\omega^{[2]}$ and linewidth $\delta\gamma^{[2]}$ changes of the CO internal stretch mode for different electron $T_e$ and lattice $T_l$ temperatures.

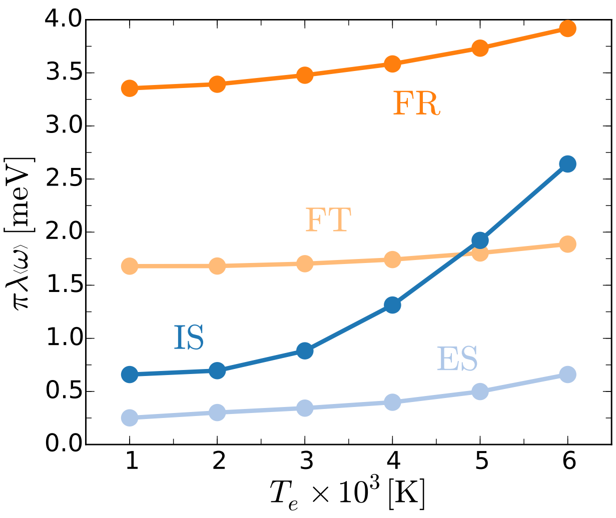


FIG. S6. The first moment of the phonon spectrum multiplied by the electron-phonon coupling constant $\lambda \langle \omega \rangle$ for each of the molecular modes (frustrated rotation and translation, external and internal stretch) and as a function of electron temperature $T_e$.

### S2.2. Mode-resolved analysis

As seen in the main text, the strongest electron-mediated vibrational mode coupling at around $t = 0.4\,\text{ps}$, i.e., when $T_e$ reaches its largest values, is that between the probed, coherent internal stretch mode ($\mathbf{q} \approx 0, \nu = \text{IS}$) and the incoherent (i.e., having finite phase) internal stretch modes ($\mathbf{q}' > 0, \nu' = \text{IS}$). When $T_l \ll T_e$ and only electron excitations around Fermi energy are considered, Eq. S12 can be approximated as [S17]

$$\pi_\nu^{[2],\text{intra}}(\omega_{0\nu}) \approx -i \frac{\pi\lambda \langle \omega \rangle}{\omega_{0\nu}} \sum_{\mu\mathbf{k}} |g_\nu^{\mu\mu}(\mathbf{k},0)|^2 \, \delta(\varepsilon_{\mu\mathbf{k}} - \varepsilon_F)\,, \qquad \text{(S15)}$$

where

$$\lambda \langle \omega \rangle = 2 \int d\Omega \alpha^2 F(\Omega; T_e) = \sum_{\mathbf{q}'\nu'} \gamma_{\mathbf{q}'\nu'}(T_e)/[\pi N_e(\varepsilon_F)\omega_{\mathbf{q}'\nu'}] \qquad \text{(S16)}$$

is the first moment of the phonon spectrum multiplied by the electron-phonon coupling constant (note that, contrary to the above equation, the Eliashberg function is usually calculated at $T_e = 0\,\text{K}$, e.g., as in Eq. S6). According to Eq. S15, $\lambda \langle \omega \rangle$ is a measure of the electron-phonon coupling entering the EMPPC term [S19, S22]. Mode-resolved data on $\lambda \langle \omega \rangle$ vs. $T_e$ can provide direct information on which modes couple predominately to the probed ($\mathbf{q} \approx 0, \nu = \text{IS}$) mode at elevated $T_e$.

The results for $\lambda \langle\omega\rangle$ resolved for each of the modes are plotted in Fig. S6 as a function of $T_e$. Clearly, at the large $T_e$ reached during the first 0.4 ps the largest increase in $\lambda \langle\omega\rangle$ corresponds to coupling with the $(\mathbf{q}' > 0, \nu' = \mathrm{IS})$ modes.

## S3. COMPUTATIONAL DETAILS

The ground state calculations are done by using the QUANTUM ESPRESSO package [S23] with a plane-wave cut-off energy of 50 Ry. Ultrasoft pseudopotentials along with the revPBE version of the GGA [S24] are used. The Brillouin zone is sampled with a $(5\times5\times1)$ Monkhorst-Pack mesh [S25]. The atomic coordinates are considered converged when the energy differences are $10^{-10}$ Ry and the forces are smaller than $10^{-4}$ Ry/$a_0$. The CO molecules are organized in the c$(2 \times 2)$ pattern with respect to the Cu(100) surface, which corresponds to a coverage of 0.5 monolayer as found in Refs. [S3, S26–S28]. The Cu(100) surface is approximated by 6 layers.

Phonon energies $\omega_\nu$ and electron-phonon coupling strengths $g_\nu$ used in Eqs. S7-S14 are obtained by means of density functional perturbation theory [S8]. The $\mathbf{k}$-summations in Eqs. S11 and S12 are performed on $(72 \times 72 \times 1)$ and $(50 \times 50 \times 1)$ Monkhorst-Pack grids, respectively. The infinitesimal parameter $\eta$ used in these equations was chosen to be 60 meV (see Refs. [S16, S17] for the physical justification and meaning of this number). The $\mathbf{q}$-summation in Eq. S12 is performed on a $(5\times5\times1)$ grid. In the main text we exclude the vertex corrections contained in Eq. S12 in order to make the numerical simulations more feasible. Nevertheless, according to Migdal's theorem the vertex corrections for electron-phonon coupling are expected to bring only a minor correction to the final phonon linewidth [S20, S29]. In order to account for surface motion in the dynamical matrix calculations, the two uppermost layers of Cu(100) are allowed to move.

The TTM input parameters (i.e., $C_e$, $C_l$, $\lambda \langle\omega^2\rangle$, and $\alpha^2 F$) are calculated by using the same computational details as listed above. Exception is the number of layers included in the dynamical matrix calculations for obtaining $\lambda \langle\omega^2\rangle$, where 5 out of 6 layers were allowed to move due to the lesser computational demand when compared to the calculation of Eq. S12. The coupled differential Eqs. S1 and S2 are solved by using the finite-difference discretization

scheme with time step of $10^{-5}$ ps and grid spacing of 1 Å.

---


[S1] P. B. Allen, Phys. Rev. Lett. **59**, 1460 (1987).

[S2] Z. Lin, L. V. Zhigilei, and V. Celli, Phys. Rev. B **77**, 075133 (2008).

[S3] T. A. Germer, J. C. Stephenson, E. J. Heilweil, and R. R. Cavanagh, J. Chem. Phys. **101**, 1704 (1994).

[S4] J. Hohlfeld, S.-S. Wellershoff, J. Gdde, U. Conrad, V. Jhnke, and E. Matthias, Chemical Physics **251**, 237 (2000).

[S5] S. Funk, M. Bonn, D. N. Denzler, C. Hess, M. Wolf, and G. Ertl, The Journal of Chemical Physics **112**, 9888 (2000).

[S6] A. M. Brown, R. Sundararaman, P. Narang, W. A. Goddard, and H. A. Atwater, ACS Nano **10**, 957 (2016).

[S7] I. Lončarić, M. Alducin, P. Saalfrank, and J. I. Juaristi, Phys. Rev. B **93**, 014301 (2016).

[S8] S. Baroni, S. de Gironcoli, A. Dal Corso, and P. Giannozzi, Rev. Mod. Phys. **73**, 515 (2001).

[S9] L. Waldecker, R. Bertoni, R. Ernstorfer, and J. Vorberger, Phys. Rev. X **6**, 021003 (2016).

[S10] P. Maldonado, K. Carva, M. Flammer, and P. M. Oppeneer, Phys. Rev. B **96**, 174439 (2017).

[S11] C. Springer, M. Head-Gordon, and J. C. Tully, Surface Science **320**, L57 (1994).

[S12] P. Saalfrank, Chem. Rev. **106**, 4116 (2006).

[S13] T. A. Germer, J. C. Stephenson, E. J. Heilweil, and R. R. Cavanagh, Phys. Rev. Lett. **71**, 3327 (1993).

[S14] L. M. Struck, L. J. Richter, S. A. Buntin, R. R. Cavanagh, and J. C. Stephenson, Phys. Rev. Lett. **77**, 4576 (1996).

[S15] F. Fournier, W. Zheng, S. Carrez, H. Dubost, and B. Bourguignon, Phys. Rev. Lett. **92**, 216102 (2004).

[S16] D. Novko, M. Alducin, and J. I. Juaristi, Phys. Rev. Lett. **120**, 156804 (2018).

[S17] D. Novko, M. Alducin, M. Blanco-Rey, and J. I. Juaristi, Phys. Rev. B **94**, 224306 (2016).

[S18] F. Giustino, Rev. Mod. Phys. **89**, 015003 (2017).

[S19] F. Marsiglio, R. Akis, and J. P. Carbotte, Phys. Rev. B **45**, 9865 (1992).

[S20] E. Maksimov and S. Shulga, Solid State Communications **97**, 553 (1996).

[S21] I. M. Lane, D. A. King, Z.-P. Liu, and H. Arnolds, Phys. Rev. Lett. **97**, 186105 (2006).

[S22] P. B. Allen and R. Silberglitt, Phys. Rev. B **9**, 4733 (1974).

[S23] P. Giannozzi, S. Baroni, N. Bonini, M. Calandra, R. Car, C. Cavazzoni, D. Ceresoli, G. L. Chiarotti, M. Cococcioni, I. Dabo, and *et al.*, Journal of Physics: Condensed Matter **21**, 395502 (2009).

[S24] Y. Zhang and W. Yang, Phys. Rev. Lett. **80**, 890 (1998).

[S25] H. J. Monkhorst and J. D. Pack, Phys. Rev. B **13**, 5188 (1976).

[S26] K.-i. Inoue, K. Watanabe, T. Sugimoto, Y. Matsumoto, and T. Yasuike, Phys. Rev. Lett. **117**, 186101 (2016).

[S27] R. Ryberg, Phys. Rev. B **32**, 2671 (1985).

[S28] M. Morin, N. J. Levinos, and A. L. Harris, The Journal of Chemical Physics **96**, 3950 (1992).

[S29] A. Migdal, JETP **7**, 996 (1958).
